# Supplementary material for: Adaptive Path Interpolation for Sparse Systems: Application to a Simple Censored Block Model
Source: arXiv:1806.05121 source file (2019-07-18)
Supplement: Supplementary file 1 [file appendix.tex]

%\section{Appendix}

%%%% -- channel symmetry --
\section{Direct proof of \eqref{eq:channelSymmetry} for symmetric distributions}
\label{proof:equi_channel_symmetry}
If $\sfx_1(-a_1) = e^{-2a_1} \sfx_1(a_1)$ holds, then we have
\begin{align*}
\int_{-\infty}^{\infty} (\tanh a_1)^{2k-1} \ \sfx_1(a_1) d a_1
	& = \int_{0}^{\infty} (\tanh a_1)^{2k-1} \ \sfx_1(a_1) da_1 - \int_{0}^{\infty} (\tanh a_1)^{2k-1} \ \sfx_1(-a_1) da_1 \\
	& = \int_{0}^{\infty} (\tanh a_1)^{2k-1} (1-e^{-2a_1}) \ \sfx_1(a_1) da_1 \\
	& = \int_{0}^{\infty} (\tanh a_1)^{2k} (1+e^{-2a_1}) \ \sfx_1(a_1) da_1 \\
	& = \int_{0}^{\infty} (\tanh a_1)^{2k} \ \sfx_1(a_1) da_1 + \int_{0}^{\infty} (\tanh a_1)^{2k} \ \sfx_1(-a_1) da_1 \\
	& = \int_{-\infty}^{\infty} (\tanh a_1)^{2k} \ \sfx_1(a_1) da_1.
\end{align*}
On the other hand, if $\int_{-\infty}^{\infty} (\tanh a_1)^{2k-1} \ \sfx_1(a_1) d a_1 = \int_{-\infty}^{\infty} (\tanh a_1)^{2k} \ \sfx_1(a_1) da_1$ holds, then we necessarily have
\begin{align*}
\sfx_1(a_1) - \sfx_1(-a_1) = \sfx_1(a_1) \tanh a_1 + \sfx_1(-a_1) \tanh a_1,
\end{align*}
which gives
\begin{align*}
\sfx_1(-a_1) = \frac{1-\tanh a_1}{1+\tanh a_1} \ \sfx_1(a_1) = e^{-2a_1} \sfx_1(a_1).
\end{align*}

\subsection{proof of \eqref{cequejaimisdeuxjoursacomprendre}}\label{elementaryapp}
\begin{lemma}
 Let $F_n: [0,1] \to \mathbb{R}_+$ be a sequence of non-negative continuous functions. Suppose that 
 $$
 \lim_{n\to +\infty} \int_0^1 d\epsilon F_n(\epsilon) = 0.
 $$
 Given any $\bar \epsilon \in [0,1]$ we can find a sequence $\epsilon_n \to \bar \epsilon$, $n\to +\infty$ such that $\lim_{n\to +\infty} F_n(\epsilon_n) =0$. 
\end{lemma}
\begin{proof}
Set $a_n = \sqrt{\int_0^1 d\epsilon F_n(\epsilon)}$. Note that $\lim_{n\to +\infty} a_n =0$. We have 
\begin{align*}
 \int_0^1 d\epsilon F_n(\epsilon) \geq \int_{\bar \epsilon - a_n}^{\bar \epsilon +a_n} F_n(\epsilon). 
\end{align*}
The mean value theorem tells us that there exists $\epsilon_n \in [\bar \epsilon - a_n, \bar \epsilon +a_n]$ such that the right hand side equals 
$2a_n F_n(\epsilon_n)$. Therefore 
\begin{align*}
 0\leq F_n(\epsilon_n) \leq \frac{1}{2} \sqrt{\int_0^1 d\epsilon F_n(\epsilon)}
\end{align*}
which implies the claim.
\end{proof}

In our application we take $F_n(\epsilon) = \mathbb{E} \left [ \< | Q_p^{K} - \< Q_p \>_{t,s; \epsilon}^K | \>_{t,s; \epsilon} \right ]$.
The whole point of this Lemma
is that although the functions $F_n$ are uniformly bounded we do not a priori know if their pointwise limit exists a.e and cannot use Lebesgue's dominated convergence theorem.

%%%% -- Rewriting the replica formula --
\subsection{Proof of \eqref{eq:RSFreeEntropy_coupled2}}
\label{proof:RSFreeEntropy_coupled2}
We copy again 
\begin{align}
\tilde{h}_{\epsilon} \big ( \underline{\sfx} \big ) 
	& = \mathbb{E} \Bigg \{ \ln \left [ \prod_{t=1}^{T} \prod_{b=1}^{l} (1 + \tanh U_b^{(t)} ) + e^{-2H} \prod_{t=1}^{T} \prod_{b=1}^{l} (1 - \tanh U_b^{(t)} ) \right ] \nonumber \\
	& \hspace{2cm} - \frac{K-1}{RT} \sum_{t=1}^{T} \ln \left [ 1 + \tanh \tilde{J} \prod_{i=1}^{K} \tanh V_i^{(t)} \right ] - \frac{1}{R} \mathbb{E}[\tilde{J}] + \frac{1}{R} \mathbb{E} [\ln \cosh \tilde{J}].
\end{align}
The first term can be rewritten as
\begin{align*}
	& \mathbb{E} \ln \left [ \prod_{t=1}^{T} \prod_{b=1}^{l} (1 + \tanh U_b^{(t)} ) + e^{-2H} \prod_{t=1}^{T} \prod_{b=1}^{l} (1 - \tanh U_b^{(t)} ) \right ] \\
	& \hspace{1cm} = \mathbb{E} \ln \left [ \prod_{t=1}^{T} \prod_{b=1}^{l} (1 + \tanh U_b^{(t)} ) \right ] + \mathbb{E} \ln \left [ 1 + e^{-2H} \prod_{t=1}^{T} \prod_{b=1}^{l} \frac{1 - \tanh U_b^{(t)} }{1 + \tanh U_b^{(t)} } \right ] \\
	& \hspace{1cm} = \mathbb{E} \ln \left [ \prod_{t=1}^{T} \prod_{b=1}^{l} (1 + \tanh U_b^{(t)} ) \right ] + \mathbb{E} \ln \left [ 1 + e^{-2  ( \sum_{t=1}^{T} \sum_{b=1}^{l} U_b^{t} + H) } \right ] \\
	& \hspace{1cm} = - \frac{K}{R} H \left ( \frac{1}{T} \sum_{t=1}^{T} \sfc \boxast (\sfx^{(t)})^{\boxast (K-1)} \right ) + \frac{K}{R} \ln 2 + H \left ( \sfh \circledast \Lambda^{\circledast} \left ( \frac{1}{T} \sum_{t=1}^{T} \sfc \boxast (\sfx^{(t)})^{\boxast (K-1)} \right ) \right )
\end{align*}
The second term can be easily seen to be
\begin{align*}
- \frac{K-1}{RT} \sum_{t=1}^{T} \ln \left [ 1 + \tanh \tilde{J} \prod_{i=1}^{K} \tanh V_i^{(t)} \right ]
	& = \frac{K-1}{RT} \sum_{t=1}^{T} H \big (\sfc \boxast (\sfx^{(t)})^{\boxast K} \big ) - \frac{K-1}{R} \ln 2.
\end{align*}
The remaining terms are
\begin{align*}
- \frac{1}{R} \mathbb{E}[\tilde{J}] + \frac{1}{R} \mathbb{E} [\ln \cosh \tilde{J}]
	& = - \frac{1}{R} \mathbb{E} \ln \left ( 1 + \tanh \tilde{J} \right ) \\
	& = \frac{1}{R} H(\sfc) - \frac{1}{R} \ln 2.
\end{align*}

%%%% -- Derivatives of free entropy --
\subsection{Proof of \eqref{eq:perturbed_f:derivative1a} and \eqref{eq:perturbed_f:derivative2b}}
\label{app:entropy-derivatives}
This appendix is essentially an extraction from \cite[Chapter 2]{Thesis:Kud:2009}.

\subsubsection{Proof of \eqref{eq:perturbed_f:derivative1a}}
We start with the same technique as we did from \eqref{eq:overlap:F-tilde1} to \eqref{eq:overlap:F-tilde2}. Let 
\begin{align*}
Z_{t,s; \epsilon}^{\sim i} := \sum_{\underline{\sigma}} \exp \left ( - \sH_{t,s}(\underline{\sigma}, \underline{\tilde{J}}, \underline{U}, \underline{m}, \underline{e}) + \sum_{\substack{k=1\\ k \neq i}}^{n} H_k \sigma_k \right ).
\end{align*}
be the partition function associated with the Gibbs expectation $\< \cdot \>_{\sim H_i}$.
With the identity
\begin{align*}
\ln \frac{Z_{t,s; \epsilon}}{Z_{t,s; \epsilon}^{\sim i}} = \ln \< e^{H_i (\sigma_i-1)} \>_{\sim H_i}
\end{align*}
and
\begin{align}
e^{H_i \sigma_i} = e^{H_i} \cdot \frac{1 + (\tanh H_i) \sigma_i}{1+\tanh H_i},
\label{eq:entropy-derivatives1}
\end{align}
we have
\begin{align}
h_{t,s;\epsilon}
	& = \frac{1}{n} \mathbb{E} \left [ \ln Z_{t,s; \epsilon}^{\sim i} \right ] + \frac{1}{n} \mathbb{E}_{\sim H_i} \left [ \ln \frac{1+(\tanh h_i)\< \sigma_i \>_{\sim H_i}}{1+\tanh H_i} \right ] \label{eq:entropy-derivatives2}
\end{align}
As $\tanh H_i$ and $\< \sigma_i \>_{\sim H_i}$ equal either 0 or 1, \eqref{eq:entropy-derivatives2} is simplified to
\begin{align*}
h_{t,s;\epsilon}
	& = \frac{1}{n} \mathbb{E} \left [ \ln Z_{t,s; \epsilon}^{\sim i} \right ] + \frac{1}{n} \epsilon_i \ln 2 \left ( 1 - \mathbb{E}_{\sim H_i} [\< \sigma_i \>_{\sim H_i}] \right ).
\end{align*}
Therefore, we have
\begin{align*}
\frac{d}{d\epsilon} h_{t,s; \epsilon} 
	& = \sum_{i=1}^{n} \frac{d}{d\epsilon_i} h_{t,s; \epsilon} \-
	= \frac{\ln 2}{n} \sum_{i=1}^{n} \left ( 1 - \mathbb{E}_{\sim H_i} [\< \sigma_i \>_{\sim H_i}] \right ).
\end{align*}

\subsubsection{Proof of \eqref{eq:perturbed_f:derivative2b}}
Let
\begin{align*}
Z_{t,s; \epsilon}^{\sim i,j} := \sum_{\underline{\sigma}} \exp \left ( - \sH_{t,s}(\underline{\sigma}, \underline{\tilde{J}}, \underline{U}, \underline{m}, \underline{e}) + \sum_{\substack{k=1\\ k \neq i,j}}^{n} h_k \sigma_k \right ).
\end{align*}
be the partition function associated with the Gibbs expectation $\< \cdot \>_{\sim H_i, H_j}$. Using again \eqref{eq:entropy-derivatives1} on the identity
\begin{align*}
\ln \left ( \frac{Z_{t,s;\epsilon}}{Z_{t,s; \epsilon}^{\sim i,j}} \right )
	& = \ln \left ( \<e^{h_i(\sigma_i-1) + h_j(\sigma_j-1)} \>_{\sim H_i, H_j} \right ),
\end{align*}
we have
\begin{align}
h_{t,s; \epsilon} = \frac{1}{n} \mathbb{E} \left [ \ln Z_{t,s; \epsilon}^{\sim i,j} \right ] + \frac{1}{n} \mathbb{E} \left [ \ln \frac{1 + \tanh H_i \< \sigma_i \>_{\sim H_i, H_j} + \tanh H_j \< \sigma_j \>_{\sim H_i, H_j} + \tanh H_i \tanh H_j \< \sigma_i \sigma_j \>_{\sim H_i, H_j}}{1 + \tanh H_i + \tanh H_j + \tanh H_i \tanh H_j} \right ]
\label{eq:entropy-derivatives3}
\end{align}
Therefore, we have
\begin{align}
\frac{1}{n} \frac{d^2}{d\epsilon^2} h_{t,s; \epsilon}
	& = \frac{1}{n} \sum_{i,j=1}^{n} \frac{d^2}{d\epsilon_j d\epsilon_i} h_{t,s; \epsilon} \label{eq:entropy-derivatives4} \\
	& = \frac{1}{n^2} \sum_{i \neq j} \frac{d^2}{d\epsilon_j d\epsilon_i} \mathbb{E} \left [ \ln \frac{1 + \tanh H_i \< \sigma_i \>_{\sim H_i, H_j} + \tanh H_j \< \sigma_j \>_{\sim H_i, H_j} + \tanh H_i \tanh H_j \< \sigma_i \sigma_j \>_{\sim H_i, H_j}}{1 + \tanh H_i + \tanh H_j + \tanh H_i \tanh H_j} \right ] \label{eq:entropy-derivatives5} \\
	& = \frac{1}{n^2} \sum_{i \neq j} \frac{d^2}{d\epsilon_j d\epsilon_i} \mathbb{E} \left [ \ln \frac{1 + \tanh H_i \< \sigma_i \>_{\sim H_i, H_j} + \tanh H_j \< \sigma_j \>_{\sim H_i, H_j} + \tanh H_i \tanh H_j \< \sigma_i \sigma_j \>_{\sim H_i, H_j}}{1 + \tanh H_i \< \sigma_i \>_{\sim H_i, H_j} + \tanh H_j \< \sigma_j \>_{\sim H_i, H_j} + \tanh H_i \tanh H_j \< \sigma_i \>_{\sim H_i, H_j} \< \sigma_j \>_{\sim H_i, H_j}} \right ] \label{eq:entropy-derivatives6} \\
	& = \frac{1}{n^2} \sum_{i \neq j} \mathbb{E}_{\sim H_i, H_j} \left [ \ln \frac{1 + \< \sigma_i \>_{\sim H_i, H_j} + \< \sigma_j \>_{\sim H_i, H_j} + \< \sigma_i \sigma_j \>_{\sim H_i, H_j}}{1 + \< \sigma_i \>_{\sim H_i, H_j} + \< \sigma_j \>_{\sim H_i, H_j} + \< \sigma_i \>_{\sim H_i, H_j} \< \sigma_j \>_{\sim H_i, H_j}} \right ]. \label{eq:entropy-derivatives6a}
\end{align}
where \eqref{eq:entropy-derivatives5} follows from $\frac{d^2}{d\epsilon_i^2} h_{t,s; \epsilon} = 0$ and substituting \eqref{eq:entropy-derivatives3} into \eqref{eq:entropy-derivatives4}, \eqref{eq:entropy-derivatives6} follows from the zero contribution of the denominator
\begin{align*}
	& \frac{d^2}{d\epsilon_j d\epsilon_i} \mathbb{E} [ \ln (1 + \tanh H_i) ] \-
	= \frac{d^2}{d\epsilon_j d\epsilon_i} \mathbb{E} [ \ln (1 + \tanh H_j) ] = 0, \\
	& \frac{d^2}{d\epsilon_j d\epsilon_i} \mathbb{E} [ \ln (1 + \tanh H_i \< \sigma_i \>_{\sim H_i, H_j}) ] \-
	= \frac{d^2}{d\epsilon_j d\epsilon_i} \mathbb{E} [ \ln (1 + \tanh H_j \< \sigma_j \>_{\sim H_i, H_j}) ] = 0.
\end{align*}
Given that $\< \sigma_S \>_{\sim H_i, H_j}$ equals either 0 or 1 for any subsets $S \subset \{ 1 \dots n\}$, one can verify the numerator and denominator of \eqref{eq:entropy-derivatives6a} can be written as
\begin{align}
	& \hspace{-0.5cm} \ln \left ( 1 + \< \sigma_i \>_{\sim H_i, H_j} + \< \sigma_j \>_{\sim H_i, H_j} + \< \sigma_i \sigma_j \>_{\sim H_i, H_j} \right ) \nonumber \\
	& = (\ln 2) (\< \sigma_i \>_{\sim H_i, H_j} + \< \sigma_i \>_{\sim H_i, H_j} + \< \sigma_i \sigma_j \>_{\sim H_i, H_j}) \nonumber \\
	& +(\ln 3 - 2\ln 2)(\< \sigma_i \>_{\sim H_i, H_j}\< \sigma_j \>_{\sim H_i, H_j} + \< \sigma_i \>_{\sim H_i, H_j} \< \sigma_i \sigma_j \>_{\sim H_i, H_j} + \< \sigma_j \>_{\sim H_i, H_j} \< \sigma_i \sigma_j \>_{\sim H_i, H_j}) \nonumber \\
	& (5\ln2 - 3\ln 3) \< \sigma_i \>_{\sim H_i, H_j} \< \sigma_j \>_{\sim H_i, H_j} \< \sigma_i \sigma_j \>_{\sim H_i, H_j} \label{eq:entropy-derivatives7}
\end{align}
and
\begin{align*}
\ln \left ( 1 + \< \sigma_i \>_{\sim H_i, H_j} + \< \sigma_j \>_{\sim H_i, H_j} + \< \sigma_i \>_{\sim H_i, H_j} \< \sigma_j \>_{\sim H_i, H_j} \right )
	& = (\ln 2) (\< \sigma_i \>_{\sim H_i, H_j} + \< \sigma_j \>_{\sim H_i, H_j}).
\end{align*}
The special case of \eqref{eq:Nishimori} in the form 
\begin{align*}
	& \mathbb{E}_{\sim H_i, H_j}[\< \sigma_i \>_{\sim H_i, H_j} \< \sigma_j \>_{\sim H_i, H_j}] = \mathbb{E}_{\sim H_i, H_j}[\< \sigma_i \>_{\sim H_i, H_j} \< \sigma_i \sigma_j \>_{\sim H_i, H_j}] \\
	& \hspace{1cm} = \mathbb{E}_{\sim H_i, H_j}[\< \sigma_j \>_{\sim H_i, H_j} \< \sigma_i \sigma_j \>_{\sim H_i, H_j}] = \mathbb{E}_{\sim H_i, H_j}[\< \sigma_i \>_{\sim H_i, H_j} \< \sigma_j \>_{\sim H_i, H_j} \< \sigma_i \sigma_j \>_{\sim H_i, H_j}]
\end{align*}
is used to simplify \eqref{eq:entropy-derivatives7} such that \eqref{eq:entropy-derivatives6a} becomes
\begin{align}
\frac{1}{n} \frac{d^2}{d\epsilon^2} h_{t,s; \epsilon}
	& = \frac{\ln 2}{n} \sum_{i \neq j} \mathbb{E}_{\sim H_i, H_j} [\< \sigma_i \sigma_j \>_{\sim H_i, H_j} - \< \sigma_i \>_{\sim H_i, H_j} \< \sigma_j \>_{\sim H_i, H_j} ].
	\label{eq:entropy-derivatives8}
\end{align}
Moreover, as $\< \sigma_i \sigma_j \> - \< \sigma_i \> \< \sigma_j \> = 0$ when $H_i$ or $H_j$ equals $\infty$, we have
\begin{align}
\mathbb{E} [\< \sigma_i \sigma_j \> - \< \sigma_i \> \< \sigma_j \> ]
	& = (1-\epsilon_i) (1-\epsilon_j) \mathbb{E}_{\sim H_i, H_j} [\< \sigma_i \sigma_j \>_{\sim H_i, H_j} - \< \sigma_i \>_{\sim H_i, H_j} \< \sigma_j \>_{\sim H_i, H_j} ].
	\label{eq:entropy-derivatives9}
\end{align}
Finally, substituting \eqref{eq:entropy-derivatives9} into \eqref{eq:entropy-derivatives8} provides \eqref{eq:perturbed_f:derivative2b}.
