# Supplementary material for: Adaptive Path Interpolation for Sparse Systems: Application to a Simple Censored Block Model
Source: arXiv:1806.05121 source file (2019-07-18)
Supplement: Supplementary file 2 [file appendixEpsilonN.tex]

%Appendix
%%% A useful remark about taking teh epsilon to zero limit 

\section{Removing the $\epsilon$-perturbation: Proof of \eqref{cequejaimisdeuxjoursacomprendre}}\label{elementaryapp}
\begin{lemma}
 Let $F_n: [0,1] \to \mathbb{R}_+$ be a sequence of non-negative continuous functions. Suppose that 
 $$
 \lim_{n\to +\infty} \int_0^1 d\epsilon F_n(\epsilon) = 0.
 $$
 Given any $\bar \epsilon \in [0,1]$ we can find a sequence $\epsilon_n \to \bar \epsilon$, $n\to +\infty$ such that $\lim_{n\to +\infty} F_n(\epsilon_n) =0$. 
\end{lemma}
\begin{proof}
Set $a_n = \sqrt{\int_0^1 d\epsilon F_n(\epsilon)}$. First we consider the case $\bar \epsilon \in ]0,1[$. Note that $\lim_{n\to +\infty} a_n =0$ so for $n$ large enough
$[\bar \epsilon - a_n , \bar \epsilon +a_n] \subset [0,1]$ and thus
\begin{align*}
 \int_0^1 d\epsilon F_n(\epsilon) \geq \int_{\bar \epsilon - a_n}^{\bar \epsilon +a_n} d\epsilon F_n(\epsilon). 
\end{align*}
The mean value theorem tells us that there exists $\epsilon_n \in [\bar \epsilon - a_n, \bar \epsilon +a_n]$ such that the right hand side equals 
$2a_n F_n(\epsilon_n)$. Therefore 
\begin{align*}
 0\leq F_n(\epsilon_n) \leq \frac{1}{2} \sqrt{\int_0^1 d\epsilon F_n(\epsilon)}
\end{align*}
which implies the claim for $\bar \epsilon \in ]0,1[$. Now we consider $\bar\epsilon =0$. Similarly as before we have for $n$ large enough
\begin{align*}
 \int_0^1 d\epsilon F_n(\epsilon) \geq \int_{0}^{a_n} d\epsilon F_n(\epsilon) = a_n F_n(\epsilon_n) 
\end{align*}
for some $\epsilon_n$ by the mean value theorem. This implies $0\leq F_n(\epsilon_n) \leq \sqrt{\int_0^1 d\epsilon F_n(\epsilon)}$ and the claim follows. The case $\bar\epsilon=1$ is treated in the same way.

\end{proof}

In our application we take $F_n(\epsilon) = \mathbb{E} \< | Q_p^{K} - \< Q_p \>_{t,s; \epsilon}^K | \>_{t,s; \epsilon}$.
The whole point of this lemma is that although the functions $F_n$ are uniformly bounded we do not a priori know if their pointwise limit exists almost everywhere and thus cannot use Lebesgue's dominated convergence theorem.
